# Supplementary material for: Substructure of Multiquark Hadrons (Snowmass 2021 White Paper)
Source: arXiv:2203.16583 source file (2022-03-30)
Supplement: Supplementary file 1 [file appendix.tex]

%{\noindent\normalfont\bfseries\Large Appendices}
\section*{Appendices}

\appendix

\section{First section of an appendix}
\label{sec:appA}

Text of Appendix A.

\section{First section of an appendix}
\label{sec:appB}

Text of Appendix B.
