# Supplementary material for: Substructure of Multiquark Hadrons (Snowmass 2021 White Paper)
Source: arXiv:2203.16583 source file (2022-03-30)
Supplement: Supplementary file 2 [file supplementary-app.tex]

\clearpage

\section{Supplementary material for ...}
\label{sec:Supplementary-App}

Not to be included with any submission

\clearpage
