# Supplementary material for: Substructure of Multiquark Hadrons (Snowmass 2021 White Paper)
Source: arXiv:2203.16583 source file (2022-03-30)
Supplement: Supplementary file 3 [file supplementary.tex]

%%%%%%%%%%%%%%%%%%%%%%%%%%%%%%%%%%%%%%%%%%%%%%%%%%%%%%%%%%%%%%%%%%%%%%%%%%%%%%%%
%%%%%%       Supplementary Material      %%%%%%%%%%%%%%%%%%%%%%%%%%%%%%%%%%%%%%%%%%%%%%%%%%%%%%%%%%
%%%%%%%%%%%%%%%%%%%%%%%%%%%%%%%%%%%%%%%%%%%%%%%%%%%%%%%%%%%%%%%%%%%%%%%%%%%%%%%%
\clearpage
\newpage
%\maketitle
%\onecolumngrid

\begin{center}
% DO NOT EDIT HERE. Instead edit macro in main.tex to keep
  \textbf{\large\normalfont\bfseries\boldmath\papertitle } \\
\vspace{0.05in}
{ \it \large Supplemental Material}\\
\vspace{0.05in}
\end{center}

%\onecolumngrid
\setcounter{equation}{0}
\setcounter{figure}{0}
\setcounter{table}{0}
\setcounter{section}{0}
%\setcounter{page}{1}
%\makeatletter

\section{First section of supplemental material}
\label{sec:suppA}

Text

\section{Second section of supplemental material}
\label{sec:suppA}

Text
